# Supplementary material for: Imaging Seebeck drift of excitons and trions in MoSe2 monolayers
Source: arXiv:2105.09617 source file (2021-05-20)
Supplement: Supplementary file 1 [file MoSe2_halos_supplementary_v3.pdf]

# Supplementary material for Imaging Seebeck drift of excitons and trions in $MoSe_2$ monolayers*

S. Park [1], B. Han [2], C. Boule [1], D. Paget [1], A. C. H. Rowe [1], F. Sirotti [1], T. Taniguchi[3], K. Watanabe[4], C. Robert [2], L. Lombez [2], B. Urbaszek [2], X. Marie [2], and F. Cadiz[1]
[1] *Physique de la matière condensée, Ecole Polytechnique, CNRS, IP Paris,91128 Palaiseau, France*
[2] *Université de Toulouse, INSA-CNRS-UPS, LPCNO, 135 Av. Rangueil, 31077 Toulouse, France*
[3]*International Center for Materials Nanoarchitectonics, National Institute for Materials Science, 1-1 Namiki, Tsukuba 305-0044, Japan and*
[4] *Research Center for Functional Materials, National Institute for Materials Science, 1-1 Namiki, Tsukuba 305-0044, Japan*

## I. LASER INDUCED PHOTODOPING EFFECTS

Figure.1 shows the PL spectrum at $T = 15K$ of the encapsulated $MoSe_2$ monolayer under a He-Ne laser excitation at 40 $\mu$W before and after being exposed for several seconds (and for the first time) to an excitation power of 9 mW. It can be seen that after high laser power exposure, the T/$X^0$ ratio exhibits a 3 fold increase, which is a signature of laser induced doping of the ML [1]. This may be due to photo-assisted charge transfer between the TMD and adsorbed molecules trapped between the hBN layers and the $MoSe_2$ [2]. After this first excitation power cycle, the T/$X^0$ remained stable after several power and cooling cycles, even with excitation powers up to 20 mW, indicating that laser induced effects only happened the first time the monolayer was exposed to high excitation power.

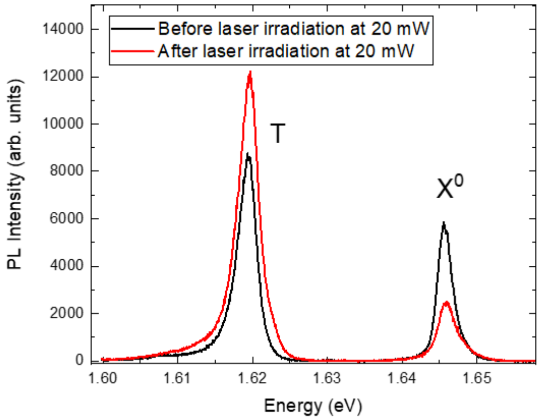


FIG. 1. PL spectrum at $T = 15$ K under a cw excitation with a He-Ne laser at 40 $\mu$W, before (black) and after (red) excitation with the same laser at 9 mW.

## II. TEMPERATURE DEPENDENCE OF THE EXCITON TRANSITION ENERGY

The temperature dependence of the neutral exciton's peak position of an hBN encapsulated $MoSe_2$ monolayer is shown in Fig.2. It reflects the temperature variation of the quasiparticle bandgap, which can be well reproduced by a three-parameter model [3] given by:

* fabian.cadiz@polytechnique.edu

$$E(T) = E(0) - S\langle\hbar\omega\rangle\left[\coth\left(\frac{\langle\hbar\omega\rangle}{2k_BT}\right) - 1\right] \tag{1}$$

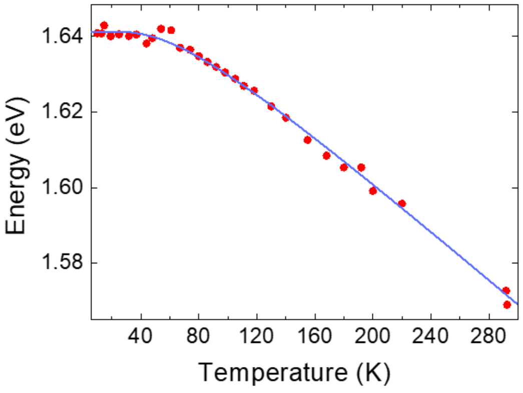


FIG. 2. Exciton's peak energy as a function of sample temperature. The continuous line correspond to a fit using Eq.(1).

Here, $E(0)$ is the exciton emission energy at 0 K, $\langle\hbar\omega\rangle$ corresponds to an averaged phonon energy, and $S$ is a dimensionless coupling constant. By fitting the measured values of the exciton peak energy for different lattice temperatures with Eq.(1), we obtained $E(0) = 1.641 \pm 0.0004$ eV, $S = 1.95 \pm 0.05$ and $\langle\hbar\omega\rangle = 15.9 \pm 0.05$ meV.

## III. POWER DEPENDENCE OF THE PL SPECTRUM

Fig.3 shows the excitation power dependence of the peak position (a) and linewidth (b) for both trion and exciton peaks under a 570 nm excitation at $T = 19$ K. The redshift of the exciton peak would correspond to a heating of the lattice up to $\sim 55$ K, according to the temperature-dependence of the PL spectrum.

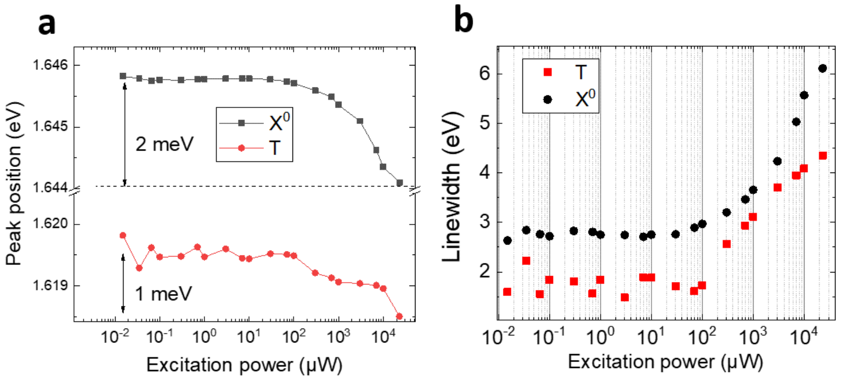


FIG. 3. (a) Peak position and (b) linewidth of trion and exciton peak as a function of excitation power.

## IV. MEASUREMENT OF THE TRION'S TEMPERATURE

As mentioned in the main text, the momentum dependence of the trion's transition energy results in an asymmetric PL emission with an exponential tail present in its low energy part [4, 5]. The trion's luminescence intensity is fitted with the following convolution :

$$I(h\nu) \propto e^{-(E^0-h\nu)/\varepsilon}\Theta\left(E^0 - h\nu\right) * g(h\nu) \tag{2}$$

where $g$ is a Lorentzian whose describing the linewidth of the transition, and $\varepsilon$ is related to the temperature $T$ of the trion gas and the ratio between the exciton ($m_X$) and the electron's mass ($m_e$). By considering that $m_X \approx 2m_e$, one finds $\varepsilon \approx 2k_bT$. Fig.4(a) shows an example of the resulting fitting at a lattice temperature of $T = 40$ K. It can be noted that the fit correctly reproduces the trion's PL energy distribution over one order of magnitude. It does not explain, however, the appereance of a slowly-decaying signal at low energies, which could be due to emission of other states such as localized trions and excitons, or to emission of hot, out-of-equilibrium trions.

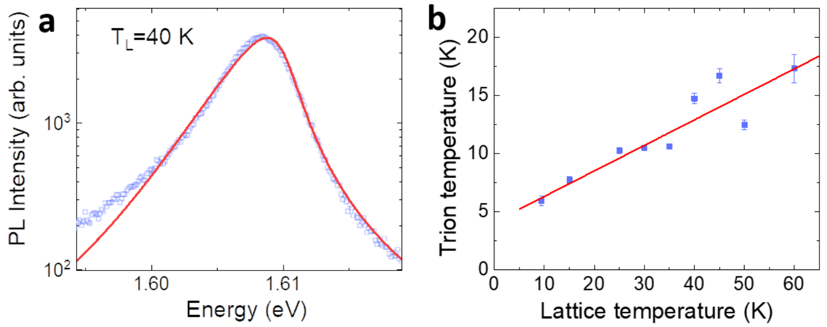


FIG. 4. (a) Trion's PL and the corresponding fit by using Eq.(2), which provides the trion temperature. (b) Trion temperature v/s lattice temperature.

In panel (b) of Fig.4 we show the extracted trion temperature $T$ as a function of the sample's temperature $T_L$. A line fit gives $T = 4.1K + 0.22T_L$. Above $T_L = 60K$, the trion's intensity in PL is too weak to be exploitable.

## V. ESTIMATION OF THE LIFETIME AND THE ABSORPTION COEFFICIENT

The absorption coefficient at resonance with the neutral exciton can be estimated to be of 5% by using the transfer matrix technique [6] . The input parameters are the thicknesses and dielectric constants of the top and bottom hBN flakes, and of the $SiO_2$ layer, as well as the linewidth of the exciton transition at low temperatures (2.6 meV) and a vacuum radiative lifetime of $\tau^0 = 2.7$ ps as recently determined [7]. In addition the model predicts an exciton radiative lifetime of 5 ps and the trion lifetime has been determined to be 140 ps at $4K$ [7]. By comparing the trion's PL intensity for a given excitation power between resonance and off resonance excitation at 570 nm, we can estimate an absorption which is 25 times smaller in the latter case.

## VI. DETERMINATION OF THE SEEBECK COEFFICIENT IN THE BOLTZMANN TRANSPORT EQUATION FORMALISM

In this section, the Seebeck coefficient is determined in a formalism based on Boltzmann's equation for a gas of conduction electrons described by a thermal distribution. In the limit of a classical gas, we can use the results of this section to describe the thermal drift of excitons and trions, albeit the open question of thermal equilibrium of excitons arises at low temperatures for which the exciton lifetime is in the ps range.

We start by writing Boltzmann's equation for the particle (exciton or trion) distribution $f$, which eventually is a function of space, time, and wavevector $k$:

$$\frac{\partial f}{\partial t} = -\vec{\nabla}_r f \cdot \frac{d\vec{r}}{dt} - \vec{\nabla}_k f \cdot \frac{d\vec{k}}{dt}$$

We now use the dynamics of a wavepacket made of Bloch states which reads $\frac{d\langle\vec{k}\rangle}{dt} = \frac{1}{\hbar}\vec{F}_t$, with $\vec{F}_t$ the force acting on the particle, which we decompose into two terms $\vec{F}_t = \vec{F}_{ext} + \vec{F}_c$. Here, $\vec{F}_{ext}$ is the external force and $\vec{F}_c$ the internal force due to collisions. We find

$$\frac{\partial f}{\partial t} = -\vec{\nabla}_r f \cdot \vec{v}_k - \vec{\nabla}_k f \cdot \frac{\vec{F}_{ext}}{\hbar} \underbrace{-\vec{\nabla}_k f \cdot \frac{\vec{F}_c}{\hbar}}_{\left(\frac{\partial f}{\partial t}\right)_c}$$

In the relaxation time approximation we suppose that collisions allows to achieve the thermodynamical equilibrium after a characteristic time $\tau$ which generally depends on $\vec{k}$. We then write $\left(\frac{\partial f}{\partial t}\right)_c = -\frac{f-f^0}{\tau(\vec{k})}$ with $f^0 = f^0(k)$ the equilibrium distribution (Fermi Dirac for trions and Bose Einstein for excitons). In steady state one finds:

$$0 = -\vec{\nabla}_r f \cdot \vec{v}_k - \vec{\nabla}_k f \cdot \frac{\vec{F}_{ext}}{\hbar} - \frac{f-f^0}{\tau(\vec{k})}$$

Finally, supposing a small departure from equilibrium, we have $\vec{\nabla}_r f \approx \vec{\nabla}_r f^0$ et $\vec{\nabla}_k f \approx \vec{\nabla}_k f^0$. The out of equilibrium distribution becomes

$$f = f^0 + \tau(\vec{k}) \left( -\vec{\nabla}_r f^0 \cdot \vec{v}_k - \vec{\nabla}_k f^0 \cdot \frac{\vec{F}_{ext}}{\hbar} \right)$$

since $f^0 = f^0(\frac{\epsilon - E_F}{k_B T}) = f^0(u)$

$$\vec{\nabla}_r f^0 = \frac{\partial f^0}{\partial u}\vec{\nabla}_r u = \frac{\partial f^0}{\partial \epsilon} \underbrace{\frac{\partial \epsilon}{\partial u}}_{k_B T} \vec{\nabla}_r (\frac{\epsilon - E_F}{k_B T}) = -k_B T \frac{\partial f^0}{\partial \epsilon} \left( \frac{1}{k_B T}\vec{\nabla}_r E_F - \frac{(E_F - \epsilon)}{k_B T^2}\vec{\nabla}_r T \right)$$

$$\vec{\nabla}_r f^0 = -\frac{\partial f^0}{\partial \epsilon} \left( \vec{\nabla}_r E_F + \frac{(\epsilon - E_F)}{T}\vec{\nabla}_r T \right)$$

and, in the other hand

$$\vec{\nabla}_k f^0 = \frac{\partial f^0}{\partial u}\vec{\nabla}_k u = \frac{\partial f^0}{\partial \epsilon} \underbrace{\frac{\partial \epsilon}{\partial u}}_{k_B T} \vec{\nabla}_k (\frac{\epsilon - E_F}{k_B T}) = \frac{\partial f^0}{\partial \epsilon}\vec{\nabla}_k \epsilon = \frac{\partial f^0}{\partial \epsilon}\hbar \vec{v}_k$$

where we have used the definition of group velocity for a wave packet $\vec{v}_k = \frac{1}{\hbar}\vec{\nabla}_k \epsilon(\vec{k})$. We obtain

$$f = f^0 + \tau(\vec{k}) \frac{\partial f^0}{\partial \epsilon} \left( \vec{\nabla}_r E_F \cdot \vec{v}_k + \frac{(\epsilon - E_F)}{T}\vec{\nabla}_r T \cdot \vec{v}_k - \vec{v}_k \cdot \vec{F}_{ext} \right)$$

In the presence of an electric field, $\vec{F}_{ext} = -e\vec{E} = e\vec{\nabla}_r \phi$ and therefore

$$f = f^0 + \tau(\vec{k}) \frac{\partial f^0}{\partial \epsilon} \left( \vec{\nabla}_r (E_F - e\phi) + \frac{(\epsilon - E_F)}{T}\vec{\nabla}_r T \right) \cdot \vec{v}_k$$

We recognize in the right hand side term the spatial gradient of the electrochemical potential, in addition to a term proportional to $\vec{\nabla}_r T$.

In reciprocal space, every quantum state occupies an elmentary volume $(2\pi)^d$ with $d$ the dimension. Since every state is double degenerate because of spin, the current density writes

$$\vec{J} = \frac{-2e}{(2\pi)^d} \int \vec{v}_k (f - f^0) d^d k$$

replacing,

$$\vec{J} = \frac{-2e}{(2\pi)^d} \int \vec{v}_k \tau(\vec{k}) \frac{\partial f^0}{\partial \epsilon} \vec{\nabla}_r (E_F - e\phi) \cdot \vec{v}_k d^d k + \frac{-e}{(2\pi)^d} \int \tau(\vec{k}) \frac{\partial f^0}{\partial \epsilon} \vec{v}_k \frac{(\epsilon - E_F)}{T} \vec{\nabla}_r T \cdot \vec{v}_k d^d k$$

In every interal, we can choose the $Ox$ axis as the axis parallel to the spatial gradient. We then find

$$\vec{J} = \underbrace{\left( \frac{-2e^2}{(2\pi)^d} \int v_x^2 \tau(\vec{k}) \frac{\partial f^0}{\partial \epsilon} d^d k \right)}_{\sigma} \vec{\nabla}_r \left( \frac{E_F - e\phi}{e} \right) + \underbrace{\left( \frac{-2e}{(2\pi)^d} \int \tau(\vec{k}) \frac{\partial f^0}{\partial \epsilon} v_x^2 \frac{(\epsilon - E_F)}{T} d^d k \right)}_{b\sigma} \vec{\nabla}_r T$$

Let us now focus on the explicit calculation of the conductivity $\sigma$. Supposing $\tau(\vec{k}) = \tau(k)$, and writing the density as $n = \frac{2}{(2\pi)^d} \int f^0 d^d k$ we find

$$\sigma = -e^2 n \frac{\int_0^{+\infty} v_x^2 \tau(k) \frac{\partial f^0}{\partial \epsilon} k^{d-1} dk}{\int_0^{+\infty} f^0 k^{d-1} dk}$$

Finally, for a parabolic dispersion $\varepsilon(k) = E_c + \hbar^2 k^2/(2m^*)$, then $dk = m/\hbar^2 d\epsilon/k$,

$$\sigma = -e^2 n \frac{\int_{E_c}^{+\infty} v_x^2 \tau(\epsilon) \frac{\partial f^0}{\partial \epsilon} (\epsilon - E_c)^{\frac{d-2}{2}} d\epsilon}{\int_{E_c}^{+\infty} f^0 (\epsilon - E_c)^{\frac{d-2}{2}} d\epsilon} = -e^2 n \frac{\frac{1}{3} \int_{E_c}^{+\infty} v^2 \tau(\epsilon) \frac{\partial f^0}{\partial \epsilon} (\epsilon - E_c)^{\frac{d-2}{2}} d\epsilon}{\int_{E_c}^{+\infty} f^0 (\epsilon - E_c)^{\frac{d-2}{2}} d\epsilon}$$

and since $v^2 = 2(\epsilon - E_c)/m*$:

$$\sigma = \frac{e^2 n}{m^*} \underbrace{\frac{-\frac{2}{3} \int_{E_c}^{+\infty} \tau(\epsilon) \frac{\partial f^0}{\partial \epsilon} (\epsilon - E_c)^{\frac{d}{2}} d\epsilon}{\int_{E_c}^{+\infty} f^0 (\epsilon - E_c)^{\frac{d-2}{2}} d\epsilon}}_{\langle \tau \rangle}$$

We find Drude's foruma $\sigma = en\mu$ avec $\mu = e\langle \tau \rangle / m^*$. Let us move now to the calculation of $b\sigma$:

$$b\sigma = \frac{-2e}{(2\pi)^d T} \int \tau(k) \frac{\partial f^0}{\partial \epsilon} v_x^2 \epsilon d^d k + \frac{E_F}{T} \underbrace{\frac{2e}{(2\pi)^d} \int \tau(k) \frac{\partial f^0}{\partial \epsilon} v_x^2 d^d k}_{-\sigma/e}$$

and so

$$b = \frac{-en}{T\sigma} \frac{\int \tau(k) \frac{\partial f^0}{\partial \epsilon} v_x^2 \epsilon d^d k}{\int f^0 d^d k} - \frac{E_F}{eT} = \frac{1}{eT} \left( \frac{\int_{E_c}^{+\infty} \tau(\epsilon) \frac{\partial f^0}{\partial \epsilon} \epsilon (\epsilon - E_c)^{\frac{d}{2}} d\epsilon}{\int_{E_c}^{\infty} \tau(\epsilon) \frac{\partial f^0}{\partial \epsilon} (\epsilon - E_c)^{\frac{d}{2}} d\epsilon} - E_F \right)$$

In summary, we find

$$\vec{J} = \sigma\vec{\nabla}_r(\frac{E_F - e\phi}{e}) + b\sigma\vec{\nabla}_r T = \sigma\vec{E} + \frac{\sigma}{e}\vec{\nabla}_r E_F + b\sigma\vec{\nabla}_r T$$

and writing $\vec{\nabla}_r E_F = \left(\frac{\partial E_F}{\partial n}\right)_T \vec{\nabla}_r n + \left(\frac{\partial E_F}{\partial T}\right)_n \vec{\nabla}_r T$

$$\vec{J} = \sigma\vec{E} + \frac{\sigma}{e}\left(\frac{\partial E_F}{\partial n}\right)_T \vec{\nabla}_r n + \frac{\sigma}{e}\left(\frac{\partial E_F}{\partial T}\right)_n \vec{\nabla}_r T + b\sigma\vec{\nabla}_r T$$

In the classical limit $\left(\frac{\partial E_F}{\partial n}\right)_T = k_B T/n$ et $\left(\frac{\partial E_F}{\partial T}\right)_n = k_B \ln(n/N_c)$

$$\vec{J} = \sigma\vec{E} + e\frac{\mu k_B T}{e}\vec{\nabla}_r n + \frac{\sigma k_B}{e}\ln\left(\frac{n}{N_C}\right)\vec{\nabla}_r T + b\sigma\vec{\nabla}_r T$$

Let us calculate $b$ in the classical limit, supposing $\tau(\epsilon) \propto (\epsilon - E_c)^r$

$$b = \frac{1}{eT}\left(\frac{\int_{E_c}^{+\infty}\frac{\partial f^0}{\partial\epsilon}\epsilon(\epsilon - E_c)^{\frac{d}{2}+r}d\epsilon}{\int_{E_c}^{\infty}\frac{\partial f^0}{\partial\epsilon}(\epsilon - E_c)^{\frac{d}{2}+r}d\epsilon} - E_F\right) = \frac{1}{eT}\left(\frac{\int_0^{+\infty}\frac{\partial f^0}{\partial u}(u + E_c)u^{\frac{d}{2}+r}du}{\int_0^{\infty}\frac{\partial f^0}{\partial u}u^{\frac{d}{2}+r}du} - E_F\right)$$

Using the identity $\int_0^{+\infty}\frac{\partial f^0}{\partial u}u^s du = -s\int_0^{+\infty} f^0 u^{s-1}du$ and the limit $f(u) \approx e^{-u/k_B T}$

$$b = \frac{1}{eT}\left(\frac{(\frac{d}{2}+r+1)\int_0^{+\infty}e^{-u/k_B T}u^{\frac{d}{2}+r}du + (\frac{d}{2}+r)E_c\int_0^{+\infty}e^{-u/k_B T}u^{\frac{d}{2}+r-1}du}{(\frac{d}{2}+r)\int_0^{\infty}e^{-u/k_B T}u^{\frac{d}{2}+r-1}du} - E_F\right)$$

$$b = \frac{1}{eT}\left((\frac{d}{2}+r+1)k_B T + E_c - E_F\right)$$

Finally, the current writes

$$\vec{J} = \sigma\vec{E} + eD\vec{\nabla}_r n + \frac{\sigma k_B}{e}\ln\left(\frac{n}{N_C}\right)\vec{\nabla}_r T + \frac{\sigma}{eT}\left((\frac{d}{2}+r+1)k_B T + E_c - E_F\right)\vec{\nabla}_r T$$

and since $E_F = E_c + k_B T\ln\left(\frac{n}{N_c}\right)$ we finally have

$$\vec{J} = \sigma\vec{E} + eD\vec{\nabla}_r n + \frac{\sigma k_B}{e}\ln\left(\frac{n}{N_C}\right)\vec{\nabla}_r T + \frac{\sigma}{eT}\left((\frac{d}{2}+r+1)k_B T - k_B T\ln\left(\frac{n}{N_c}\right)\right)\vec{\nabla}_r T$$

$$\vec{J} = \sigma\vec{E} + eD\vec{\nabla}_r n + \sigma\underbrace{(\frac{d}{2}+r+1)\frac{k_B}{e}}_{S}\vec{\nabla}_r T$$

We find the Seebeck coefficient

$$S = \left(\frac{d}{2}+r+1\right)\frac{k_B}{e}$$

## VII. MODELING OF TRION AND EXCITON HALO EFFECTS

Modeling drift-diffusion of charged particles in semiconductors uses the Van Roosbroeck set of coupled differential equations. Although these equations describe conduction electrons and valence holes, we will adapt them in the next subsection for the modeling of excitons and trions.

The first is Poisson's equation:

$$\nabla \cdot (\epsilon \nabla \psi) = q\left(C + p - n\right), \tag{3}$$

where $n$ and $p$ are the total electron and hole concentrations respectively, $C$ is the doping density of which the sign determines whether the semiconductor is n-type or p-type, $q$ is the absolute value of the electronic charge, $\epsilon$ is the dielectric permittivity, and $\psi$ is the electrostatic potential. The second is the continuity or transport equation for electrons:

$$\nabla \cdot \vec{j}_n = qR - qG \tag{4}$$

where $R$ is a net recombination rate and $G$ is the net generation rate of electron-hole pairs. The electron current density in Eq. (4) is given by

$$\vec{j}_n = -q\mu_n n \nabla \phi_n \tag{5}$$

where $\mu_n$ is the electron mobility and $\phi_n$ is the quasi-electrochemical potential for electrons. Similarly for holes the continuity equation reads:

$$\nabla \cdot \vec{j}_p = qG - qR \tag{6}$$

where

$$\vec{j}_p = -q\mu_p p \nabla \phi_p. \tag{7}$$

The recombination rate $R$ usually includes three possible recombination routes. Spontaneous radiative recombination across the bandgap is

$$R_{\text{spont}} = r_{\text{spont}}\left(np - n_i^2\right) \tag{8}$$

where $n_i$ is the intrinsic concentration and $r_{\text{spont}}$ is a scalar coefficient. The second is Shockley-Read-Hall (SRH) recombination:

$$R_{\text{SRH}} = \frac{\left(np - n_i^2\right)}{(n + n_1)\tau_p + (p + p_1)\tau_n}, \tag{9}$$

where $n_1$ and $p_1$ are the characteristic electron and hole concentrations, and $\tau_n$ and $\tau_p$ are the SRH electron and hole lifetimes. The last recombination term is the Auger process:

$$R_{\text{Auger}} = \left(np - n_i^2\right)\left(C_n n + C_p p\right) \tag{10}$$

where $C_n$ and $C_p$ are the electron and hole Auger coefficients. Since these three routes are independent the total recombination rate is

$$R = R_{\text{spont}} + R_{\text{SRH}} + R_{\text{Auger}}. \tag{11}$$

The final missing ingredient is the charge carrier statistics. In the degenerate limit full Fermi-Dirac statistics should be used, but in the classical limit we have the usual expressions for the electron and hole concentrations. Respectively, they are

$$n = N_c \exp\left(\frac{\psi - \phi_n - E_g}{k_B T}\right) \tag{12}$$

and

$$p = N_v \exp\left(\frac{\phi_p - \psi}{k_B T}\right) \tag{13}$$

where $T$ is the temperature and $k_B$ is Boltzmann's constant. $N_c$ and $N_v$ are the effective densities-of-state for the conduction and valence bands respectively.

Equations (3), (4) and (6) are the Van Roosbroeck equations which are solved numerically for $\psi$, $\phi_n$ and $\phi_p$ for any desired set of boundary conditions. This is typically done using the so-called Scharfetter-Gummel discretization which ensures current conservation. In this way transport characteristics, including the opto-electronic properties of a range of semiconductors and semiconductor devices can be calculated.

### A. Adapting the Van Roosbroeck equations for Exciton and Trion transport

Modeling the drift-diffusion of trions and excitons requires modifications to the usual Van Roosbroeck equations. Trions and excitons are not present in equilibrium unlike electrons and holes, and they diffuse (or drift in the case of trions) independently of other quasi-particles i.e. the transport is unipolar. These two aspects are accounted for in the model by artificially using a large background doping level. Either donors or acceptors can be chosen, and here we choose to use acceptors so that

$$n_0 \ll n_i \ll p_0 \tag{14}$$

where the '0' subscript indicates the equilibrium concentration. The acceptor concentration is chosen to be sufficiently large that, in the excitation power range of interest, $\Delta n$ the photo-excited carrier density is much large than $n_0$ so that the following is true:

$$n_0 \ll \Delta n = \Delta p \ll p_0 \approx -C. \tag{15}$$

Thus the hole concentration as modeled is constant, independent of the photo-excitation, and the electron concentration is essential made up of photo-electrons.

Another consequence of Eq. (15) is that $C + p - n = C + p_0 + \Delta p - n_0 - \Delta n \approx 0$ on the right hand side of Eq. (3). This ensures that any possible electrostatic couplings to oppositely charged particles (i.e. space charge effects) are absent. This should be the case, even for trions, which exist in the absence of oppositely charged particles.

In the following therefore the "electrons" represent the particles whose transport is of interest i.e. trions or excitons, and "hole" transport is negligible.

### B. Inclusion of the Seebeck effect

Thermal effects on transport can be included in an extended version of the Van Roosbroeck equations where a fourth (heat) transport equation is added and the temperature becomes a fourth independent variable. This is not the approach used here. Rather the temperature gradient and the Seebeck effect is imposed upon the currents so that Eq. (5) and Eq. (7) become:

$$\vec{j}_n = -n\mu_n q \left(\nabla\phi_n + S_n \nabla T\right) \tag{16}$$

and

$$\vec{j}_p = -p\mu_p q \left(\nabla\phi_p + S_p \nabla T\right) \tag{17}$$

where $S_n$ and $S_p$ are the electron and hole Seebeck coefficients respectively.

As mentioned in Section VII A, the model used here must be adapted so that the "hole" current is negligibly small. For this reason $S_p = 0$ is chosen so that, regardless of the temperature gradient which is imposed on the problem, the Seebeck current of holes is zero.

The last point to note is that because trions and excitons are not thermally excited quasi-particles, the Boltzmann carrier statistics used for true electrons and holes should not be applied. The temperature gradient that is applied to the problem based on estimations from the trion line shape is therefore not applied to a re-calculation of the "electron" density, and is used only in the calculation of the Seebeck current. In other words since we are only interested in photo-excited particles, the absolute value of the temperature is irrelevant to the problem.

The form of the temperature gradient can be estimated from the data, and is approximated here by a Gaussian consistent with expectation for laser absorption in solids [8]. The width of the Gaussian is taken to be $5\sigma$ where $\sigma$ is the width of the Gaussian laser excitation to be presented in Section VII D. The variation with laser power is also estimated from the data and is here approximated by an erf function. Consequently the temperature is given by

$$T(r, P) = 1.35 T_L \mathrm{erf}\left(\frac{P}{8 \times 10^{-3}}\right) \exp\left(-\frac{r^2}{(5\sigma)^2}\right) + T_L, \tag{18}$$

where $T_L$ is the background lattice temperature. An example of the resulting temperature gradient curves is shown for selected (high) powers in Fig. 5.

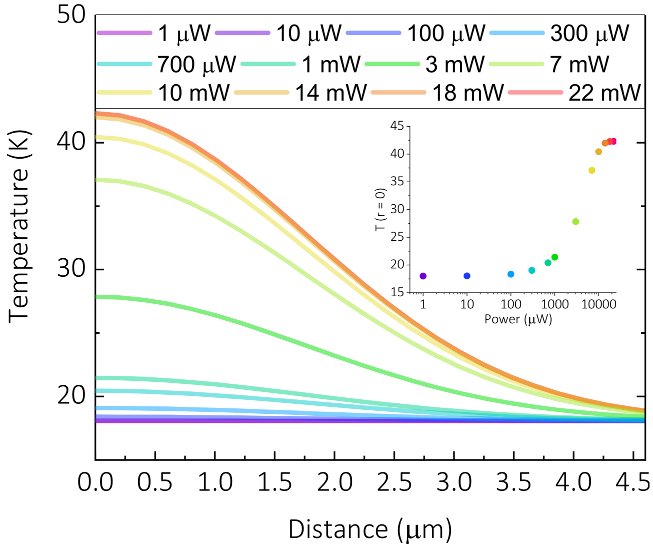


FIG. 5. Gaussian temperature gradients for selected excitation powers imposed when calculating the numerical solution of Eq. 19. The erf variation in the temperature at $r = 0$ is shown inset.

### C. Effective transport equation for trions and excitons

The assumptions and simplifications made in Sections VII A and VII B yields an effective transport equation given by:

$$\nabla \cdot \{-\mu\, \delta c\, (\nabla \phi + S \nabla T)\} = \frac{\delta c}{\tau} + C \delta c^2 - G, \tag{19}$$

where the "n" subscripts from the previous sections have been dropped to avoid confusion. $\delta c$ is then the particle concentration, $\mu$ the particle mobility, $S$ the particle's Seebeck coefficient, $C$ the particle's Auger coefficient and $\tau$ its lifetime.

In what follows the particle lifetimes will be taken from the literature, $\tau = 140$ ps for trions, and $\tau = 5$ ps for excitons, and the Auger coefficient in both cases will be set to its upper expected limit, $C = 0.1$ cm$^2$/s. These are considered to be non-adjustable parameters.

### D. Excitation profile

The excitation dynamics of trions and excitons is assumed to occur in two steps. The first step is the creation of electron/hole pairs (or hot excitons) with a generation profile given by the Gaussian laser excitation spot:

$$G(r, P) = P \frac{\lambda \alpha}{\pi \mathrm{hc} \sigma^2} \exp(-\alpha d) \exp\left(-\frac{r^2}{\sigma^2}\right), \tag{20}$$

where $P$ is the laser power, $\lambda = 570$ nm the light wavelength, $\alpha = 6.5 \times 10^3$ $\mu$m$^{-1}$ is the inverse absorption length chosen so that approximately 0.15 % of the non-resonant excitation is absorbed in the $d = 1$ nm thick sample, h is Planck's constant and c is the speed of light. The parameter $\sigma = 0.5$ $\mu$m is the experimentally measured size of the Gaussian excitation spot.

The resulting excited population has time to diffuse prior to the formation of trions and excitons which takes approximately 18 ps. In the model, a bare hot exciton diffusion length is chosen so that the steady-state profile is close to that of the low power trion and exciton profiles (which are very similar). Fig. 6 shows both the true Gaussian profile of the laser which creates hot excitons (solid curve), and the steady-state bare hot exciton profile obtained at very low powers (dashed curve). The dashed curve is then used as the profile of the generation term in Eq. (19) which models trion and exciton transport.

With regards to the amplitude of the generation term in Eq. (19), in the case of excitons the normalized profile shown as the dashed line in Fig. 6 is multiplied by the same pre-factor as Eq. (20) i.e. $P\lambda\alpha/\pi hc\sigma^2 \exp(-\alpha d)$. In

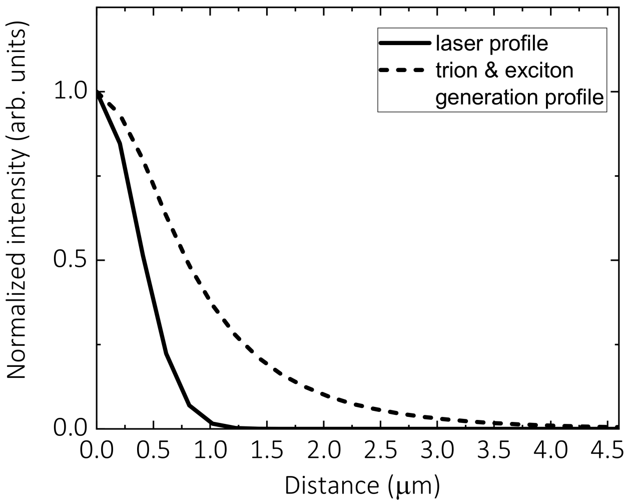


FIG. 6. Generation profiles. The solid, black line shows that Gaussian laser profile use to generate hot electron/hole pairs. The blacked, dashed line is the resulting steady-state profile obtained by solving the Van Roosbroeck equations for a very low excitation power. This black, dashed line is used as the generation profile for the trions and excitons.

the case of trions, generation is limited by the quantity of free charge available in equilibrium, and this is empirically accounted for by modifying this pre-factor to read

$$\min\left(P, 400\times 10^{-6}\right)\frac{\lambda\alpha}{\pi h c\sigma^2}\exp\left(-\alpha d\right). \tag{21}$$

Physically, for incident powers above 400 $\mu$W no supplementary trions are created. Note however that further increases in power will still affect the temperature gradient according to the discussion in Section VII B.

### E. Trion and Exciton Seebeck effect

Figure 7 shows the trion profiles obtained for a Seebeck coefficient, $S$ = 300 $\mu$V/K, and a trion mobility of 100 $cm^2$/Vs. The qualitative agreement with the experimental data is excellent and indicates that the observed halo effect is indeed due to a trion Seebeck effect.

The model also indicates that Auger recombination is negligible, even at the highest excitation powers. Fig. 8 shows the profiles for the radiative and Auger rates for an excitation power of 22 mW i.e. the red curve in Fig. 7. The calculation shows that at this power the trion concentration at the excitation spot is 2.7× $10^{10}$ $cm^{-2}$ so that the radiative recombination rate is $\delta c/\tau = 1.9\ \times 10^{20}$ $cm^{-2}s^{-1}$, and the Auger recombination rate is $C\delta c^2 = 7.2\times 10^{19}$ $cm^{-2}s^{-1}$ as can be seen at a distance of 0 $\mu$m in Fig. 8. Clearly, at larger distances from the excitation spot the density decreases due to recombination occurring during transport and the Auger route become progressively less important. As such the radiative profile (which is measured experimentally) follows the particle density profile.

It should be noted that the reason the Auger is negligible for trions is because their presence is generation limited according to Eq. (21). The observed strong saturation in the trion line intensity at high powers is therefore generation limited, and not Auger limited. The model also reproduces well this strong saturation at high powers as seen in Fig. 10.

In order to obtain profiles for the excitons, the lifetime is reduced to its known value of 5 ps, and a mobility that accounts for the effective mass difference with the trion is used i.e. $\mu$ = 150 $cm^2$/Vs. The sole adjustable parameter is the Seebeck coefficient. Figure 9 shows the exciton profiles obtained for a Seebeck coefficient, $S$ = 400 $\mu$V/K. In order to obtain the correct integrate intensity of the exciton line with respect to that of the trions a reduction by a factor of 15 is required in the generation term for excitons relative to trions (i.e. in Eq. (20)). When this is done the integrated intensity curves shown in Fig. 10 are obtained.

In Fig. 10 the trion curve shows a relatively strong saturation due to the limitation on trion generation imposed by the equilibrium carrier concentration via Eq. (21). The exciton curve is essentially linear over the whole power range, with a very weak downturn at the highest powers due to the onset of Auger recombination. Fig. 10 agrees well with the observed, integrated luminescence intensity dependence on excitation power.

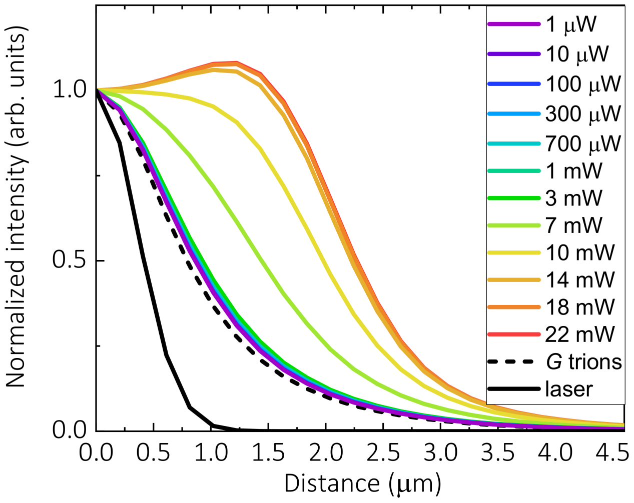


FIG. 7. Trion line profiles as a function of excitation power obtained using the model parameters outlined in the text. The black lines correspond to those shown for the excitation profiles in Fig. 6

.

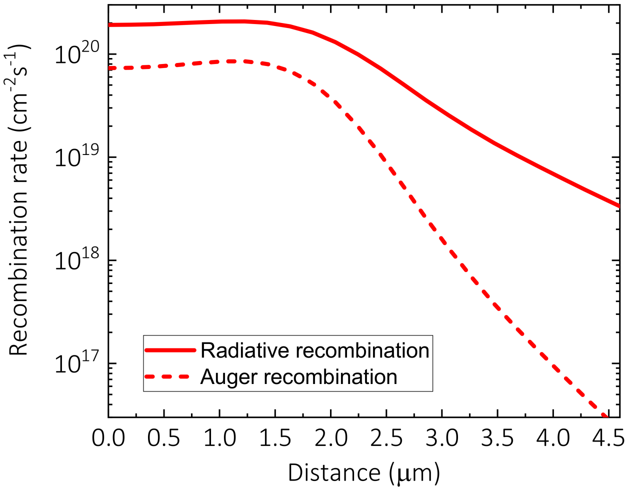


FIG. 8. Profiles of the radiative and Auger recombination rates for trions for an excitation power of 22 mW. The limit on trion generation imposed by the concentration of free equilibrium charge carriers strongly limits the trion density at high powers as shown in Fig. 10, and as observed experimentally. Consequently, Auger recombination is negligible for all powers, even at the excitation spot.

.

---


[1] F. Cadiz, C. Robert, G. Wang, W. Kong, X. Fan, M. Blei, D. Lagarde, M. Gay, M. Manca, T. Taniguchi, K. Watanabe, T. Amand, X. Marie, P. Renucci, S. Tongay, and B. Urbaszek, Ultra-low power threshold for laser induced changes in optical properties of 2D molybdenum dichalcogenides, 2D Materials **3**, 045008 (2016).

[2] T. Venanzi, H. Arora, A. Erbe, A. Pashkin, S. Winnerl, M. Helm, and H. Schneider, Exciton localization in MoSe2 monolayers induced by adsorbed gas molecules, Applied Physics Letters **114**, 172106 (2019).

[3] K. O'Donnell and X. Chen, Temperature dependence of semiconductor band gaps, Applied Physics Letters **58**, 2924 (1991).

[4] J. W. Christopher, B. B. Goldberg, and A. K. Swan, Long tailed trions in monolayer MoS2: Temperature dependent asymmetry and resulting red-shift of trion photoluminescence spectra, Scientific Reports **7**, 14062 (2017).

[5] Y. Zhumagulov, A. Vagov, D. R. Gulevich, P. E. Faria Junio, and V. Perebeinos, Trion induced photoluminescence of a doped MoS2 monolayer, J. Chem. Phys. **153**, 044132 (2020).

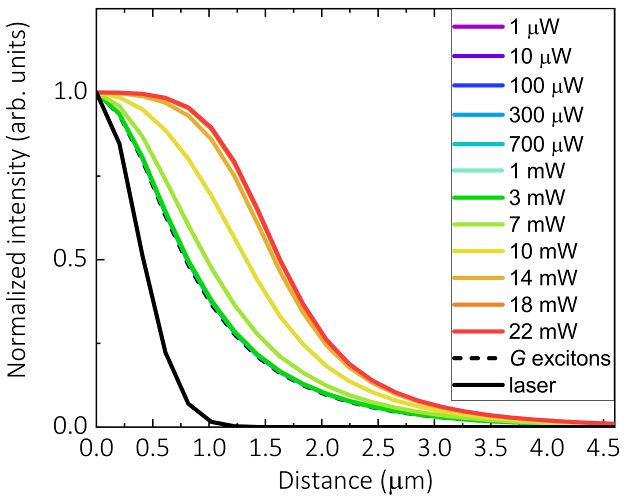


FIG. 9. Exciton line profiles as a function of excitation power obtained using the model parameters outlined in the text.

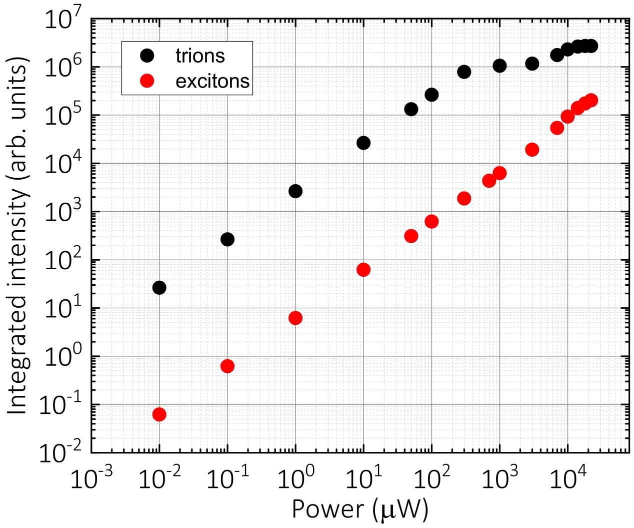


FIG. 10. The power dependence of the trion and exciton intensities which shows the saturation in the trion intensity due to the limit imposed by the availablility of equilibrium charge carriers implemented by Eq. (21).


[6] C. Robert, M. Semina, F. Cadiz, M. Manca, E. Courtade, T. Taniguchi, K. Watanabe, H. Cai, S. Tongay, B. Lassagne, P. Renucci, T. Amand, X. Marie, M. Glazov, and B. Urbaszek, Optical spectroscopy of excited exciton states in MoS2 monolayers in van der waals heterostructures, Physical Review Materials **2**, 011001(R) (2018).

[7] H. H. Fang, B. Han, C. Robert, M. A. Semina, D. Lagarde, E. Courtade, T. Taniguchi, K. Watanabe, T. Amand, B. Urbaszek, M. M. Glazov, and X. Marie, Control of the exciton radiative lifetime in van der waals heterostructures, Physical Review Letters **123**, 067401 (2019).

[8] P. Loza, D. Kouznetsov, and R. Ortega, Temperature distribution in a uniform medium heated by linear absorption of a gaussian light beam, Applied Optics **33**, 3831 (1994).
